# Supplementary material for: On Episodes, Prototypical Networks, and Few-shot Learning
Source: arXiv:2012.09831 source file (2021-11-30)
Supplement: Supplementary file 1 [file appendix_experiments.tex]

\subsection{Implementation details}
\label{sec:appendix_benchmarksetup}

\mypar{Benchmarks.}
In our experiments, we use three popular FSL benchmarks.
\textbf{\textit{mini}ImageNet}~\citep{vinyals2016matching} is a subset of ImageNet generated by randomly sampling 100 classes, each with 600 randomly sampled images.
We adopt the commonly used splits of~\citet{ravi2016optimization} who use 64 classes for meta-training, 16 for meta-validation and 20 for meta-testing.
\textbf{CIFAR-FS} was proposed by~\citet{bertinetto2019meta} as an anagolous version of \textit{mini}Imagenet for CIFAR-100.
It uses the same sized splits and same number of images per split as
\emph{mini}ImageNet.
\textbf{\textit{tiered}ImageNet}~\citep{ren2018meta} is also constructed from ImageNet, but contains 608 classes, with 351 training classes, 97 validation classes and 160 test classes.
The class split have been generated using WordNet \citep{miller1995wordnet} to ensure that the training classes are semantically ``distant'' to the validation and test classes.
For all datasets, we use images of size $84{\times}84$.

\mypar{Architecture.}
In all our experiments, $f_\theta$ is represented by a ResNet12 with widths $[64, 160, 320, 640]$.
We chose this architecture, initially introduced by~\citet{lee2019meta}, as it is the one which is most frequently adopted by recent FSL methods.
Unlike most methods, we do not use a DropBlock regulariser~\citep{ghiasi2018dropblock}, as we did not notice it to meaningfully contribute to performance.

\mypar{Optimisation.}
To train all the models used for our experiments, unless differently specified, we used a SGD optimiser with Nesterov momentum, weight decay of 0.0005 and initial learning rate of $0.1$.
For \textit{mini}ImageNet and CIFAR-FS we decrease the learning rate by a factor of 10 after 70\% of epochs have been trained, and train for a total of 120 epochs.
As data augmentations, we use random horizontal flipping and centre cropping.

Only for the experiments of Sec.~\ref{sec:SOTA}, we slightly change our training setup.
On CIFAR-FS, we increase the number of training epochs from 120 to 240, which improved accuracy of about 0.5\%.
For \textit{tiered}ImageNet, we train for 120 epochs and decrease the learning rate by a factor of 10 after 50\%  and 75\% of the training progress.
For \textit{tiered}ImageNet only we increased the batch size to 1024, and train on 64 classes and 16 images per class within a batch, as we found it being beneficial.
For the other datasets it did not improve performance.
These changes affect all our methods and baselines: NCA, Prototypical Networks (with both old and new batch setup), and SimpleShot~\citep{wang2019simpleshot}.

\mypar{Projection network.}
Similarly to~\citep{khosla2020supervisedcontrastive,chen2020simple}, we also experimented (for both \pn and NCA) with a \textit{projection network} (but \emph{only} for the comparison of Sec.~\ref{sec:SOTA}).
The projection network is a single linear layer $A \in \mathbb{R}^{M \times P}$ that is placed on top of $f_{\theta}$ at training time, where $M$ is the output dimension of the neural network $f_{\theta}$ and $P$ is the output dimension of $A$, which can be considered as a hyper-parameter.
The output of $A$ is only used during training.
At test time, we do not use the output of $A$ and directly use the output of $f_{\theta}$.
For CIFAR-FS and \textit{tiered}ImageNet, we found this did not help performance.
For \textit{mini}ImageNet however we found that this improved performance, and we set $P=128$ (which worked best for both \pn and NCA).
Note that this is not an unfair advantage over other methods.
Compared to SimpleShot~\citep{wang2019simpleshot} and other simple baselines, we actually use fewer parameters without the projection network (effectively making our ResNet12 a ResNet11) since they use an extra fully connected layer to minimise cross entropy during pre-training.

\subsection{Choice of hyper-parameters}\label{sec:hyperparameter}
\begin{table}[t]
\centering
\begin{footnotesize}
  \begin{tabular}{@{}ccccc@{}}

                                      & \multicolumn{2}{c}{\textit{mini}ImageNet}         & \multicolumn{2}{c}{CIFAR-FS}      \\    \toprule
    \textbf{method}                       & \textbf{1-shot}        & \textbf{5-shot}   & \textbf{1-shot}  & \textbf{5-shot} \\ \midrule
    \textbf{\pn (SimpleShot)}	& $57.99 \pm 0.21 $	& $74.33 \pm 0.16 $ & 	$53.76 \pm 0.22$& 	$68.54 \pm 0.19$\\
\textbf{\pn (ours)}& 	$62.79 \pm 0.12$& 	$78.82 \pm 0.09$& 	$59.60 \pm 0.13$	& $74.64 \pm 0.11$ \\
\midrule
\textbf{NCA (SimpleShot)}	& $61.21 \pm 0.22$	& $76.39 \pm 0.16$	& $59.41 \pm 0.24$ & 	$73.29 \pm 0.19$ \\
\textbf{NCA (ours)}	& $64.94 \pm 0.13$	& $80.12 \pm 0.09 $	& $62.07 \pm 0.14$& 	$76.26 \pm 0.10$

\end{tabular}%
%}
\end{footnotesize}
    \vspace{0.3cm}
		\caption{\small{Comparison (on the validation set of \textit{mini}ImageNet and CIFAR-FS) between using the hyper-parameters from SimpleShot~\citep{wang2019simpleshot} and the ones from this paper (\textbf{ours}). Models have been trained with batches of size 256, as in~\citep{wang2019simpleshot}.
\pn's episodic batch setup uses $a{=}16$, as it is the highest performing one.}}
\label{tab:simple_shot_schedule}
\end{table}

During the experimental design, we wanted to ensure a fair comparison between the NCA and PNs.
As a testimony of this effort, we obtained very competitive results for PNs (see for example the comparison to recent papers where architectures of similar capacity were used~\citep{wang2019simpleshot,chen2019closer}).
In particular:
\begin{tight_it}
\item We always use the normalisation strategy of~\citet{wang2019simpleshot}, as it is beneficial also for PNs.
\item Unless expressively specified, we always used PNs’ 5-shot model, which in our implementation outperforms the 1-shot model (for both 1-shot and 5-shot evaluation).
Instead, \citep{snell2017prototypical} train and tests with the same number of shots.
\item Apart from the episodes hyper-parameters of PNs, which we did search and optimise over to create the plots of Fig.~\ref{fig:plots-batch}, the only other hyper-parameters of PNs are those related to the training schedule, which are the same as the NCA. To set them, we started from the simple SGD schedule used by~\citet{wang2019simpleshot} and only marginally modified it by increasing the number of training epochs to 120, increasing the batch size to 512 and setting weight decay and learning rate to $5e-4$ and $0.1$, respectively.
As a sanity check, we trained both the NCA and PNs with the exact training schedule used by~\citet{wang2019simpleshot}.
Results are reported in Table~\ref{tab:simple_shot_schedule}, and show that the schedule we used for this paper is considerably better for both PNs and NCA.
In general, we observed that the modifications were beneficial for both NCA and PNs, and improvements in performance in NCA and PNs were highly correlated. This is to be expected given the high similarity between the two methods and losses.
\end{tight_it}

\subsection{Additional results for Sec.~\ref{sec:expm_batch_size}}
\label{sec:plots-batch-appendix}
Fig.~\ref{fig:plots-batch-appendix} complements the results of Fig.~\ref{fig:plots-batch} from Sec.~\ref{sec:expm_batch_size}
\begin{figure*}[t]
\centering
\includegraphics[width=0.40\textwidth]{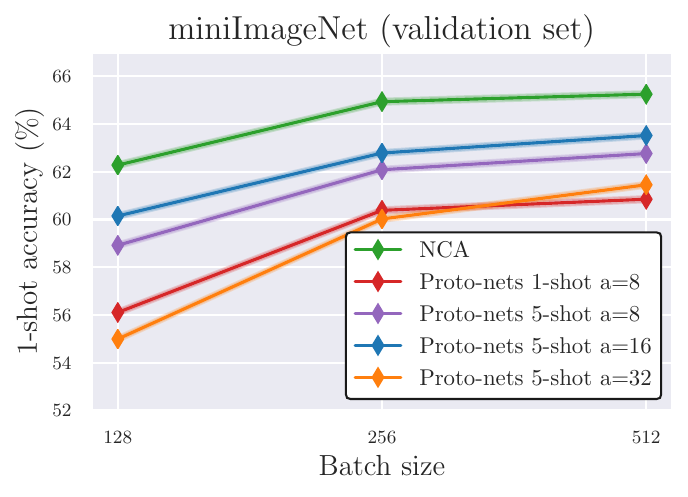}
\includegraphics[width=0.40\textwidth]{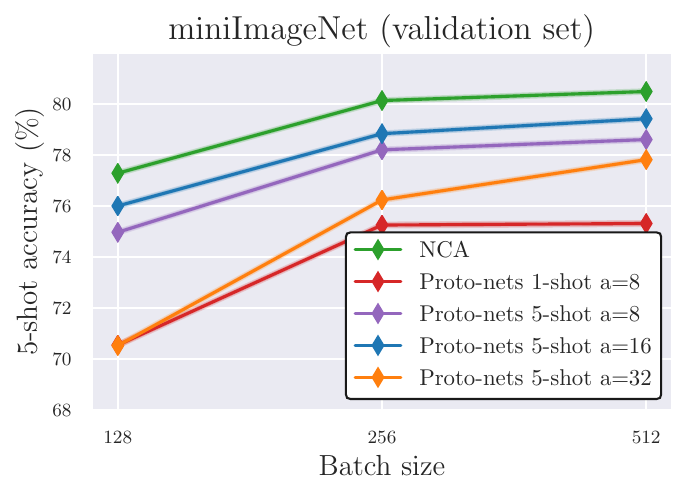}
\caption{\small{1-shot and 5-shot accuracies on the validation set of \textit{mini}ImageNet for different batch sizes.
Models are trained using NCA or PNs with different configurations: 1-shot with $a=8$ and 5-shot with $a=8$, $16$ or $32$.
Reported values correspond to the mean accuracy of five models trained with different random seeds.
Shaded areas represent 95\% confidence intervals.
Please see Sec.~\ref{sec:expm_batch_size} for details.
}
\label{fig:plots-batch-appendix}
}
\end{figure*}

\subsection{Details about number of pairs description of Section~\ref{sec:nca}}
\label{sec:appendix_pairs}
In this section we demonstrate that the total number of training pairs that NCA can exploit within a batch is always strictly superior than the one exploited by the episodic batch strategy used by Prototypical Networks.

To ensure we have a ``valid'' episodic batch with a nonzero number of both positive and negative distance pairs, we assume that $n, m \geq 1$, and $w \geq 2$.

Below, we show that the number of positives for NCA, \ie ${m+n \choose 2} w$, is always greater or equal than the one for PNs, which is $mnw$:

\begin{align*}
  {m+n\choose2} w & = \frac{(m+n)!}{2!(m+n-2)!} w \\
               & = \frac{1}{2}(m+n)(m+n-1) w \\
               & = \frac{1}{2}(m^2 + 2mn - m + n^2 - n) w \\
               & = \frac{1}{2}(m(m-1) + 2mn + n(n-1)) w\\
               & \geq \frac{1}{2}(2mn) w = wmn.
\end{align*}

Similarly, we can show for negative distance pairs that ${w\choose2} (m+n)^2 > w(w-1)mn$:

\begin{align*}
  {w\choose2} (m+n)^2 & = \frac{w!}{2!(w-2)!} (m^2 + 2mn + n^2) \\
                      & = \frac{1}{2}w(w-1) (m^2 + 2mn + n^2) \\
                      & > \frac{1}{2}w(w-1)(2mn) \\
                      & = w(w-1)mn.
\end{align*}

This means that the NCA has at least the same number of positives as Prototypical Networks, and always has strictly more negative distances.

The total number of \emph{extra} pairs that NCA can rely on is $\frac{w}{2}(w(m^2+n^2) - m - n)$.

\subsection{Details about number of pairs description of Section~\ref{sec:expm_batch_size}}
\label{sec:appendix_pairs_batch_size}
\begin{table}[t]
\centering
\resizebox{0.5\textwidth}{!}{%
\begin{tabular}{@{}rlrrr@{}}
\toprule
\multicolumn{1}{l}{\textbf{rank}} & \textbf{method} & \multicolumn{1}{l}{\textbf{\# pos}} & \multicolumn{1}{l}{\textbf{\# neg}} & \multicolumn{1}{l}{\textbf{\# total pairs}} \\ \midrule
1                                 & \textit{NCA}             & 1792                                & 129024                              & 130816                                      \\
2                                 & \textit{5-shot a=16}     & 1760                                & 54560                               & 56320                                       \\
3                                 & \textit{5-shot a=8}      & 960                                 & 60480                               & 61440                                       \\
4                                 & \textit{5-shot a=32}     & 2160                                & 32400                               & 34560                                       \\
5                                 & \textit{1-shot a=8}      & 448                                 & 28224                               & 28672                                       \\ \bottomrule
\end{tabular}%
}
\caption{\small{Number of positives and negatives used in the experiments of Fig.~\ref{fig:plots-batch} with batch size 512.}}
\label{tab:batch_size_pairs}
\end{table}

In Table~\ref{tab:batch_size_pairs} we plot the number of positives and negatives (gradients contributing to the loss) for the NCA and different episodic configurations of PNs, to see whether the difference in performance can be explained by the difference in the number of distance pairs that can be exploited in a certain batch configuration.
This is often true, as
the ranking can almost be fully explained by the number of total pairs in the right column.
However, there are two exceptions to this: 5-shot with a=16 and 5-shot with a=8.

To understand this, we can see that the number of positive pairs is much higher for a=16 than for a=8.
Since the positive pairs constitute a less frequent (and potentially more informative) training signal, this can explain the difference.
The a=32 variant has an even higher number of positives than a=16, but the loss in performance there could be explained by a drastically lower number of negatives, and by the fact that the number of ways used during training is lower.
So, while indeed generally speaking the higher number of pairs the better (which is also corroborated by Fig.~\ref{fig:plots-posnegsample}, where moving right on the x-axis sees higher performance for both NCA and PNs), one should also consider how this interacts with the positive/negative balance and the number of classes present within a batch.

%%% Local Variables:
%%% mode: latex
%%% TeX-master: "main"
%%% End:
